# Supplementary material for: An electrical molecular motor driven by angular momentum transfer
Source: arXiv:2503.05351 source file (2025-03-07)

7.543 7.540 7.527 7.525 7.421 7.418 7.406 7.403 7.391 7.388 7.376 7.373 7.361 7.358 7.346 7.343 7.267 7.265 7.253 7.250 7.240 4.344 4.324 4.192 4.171

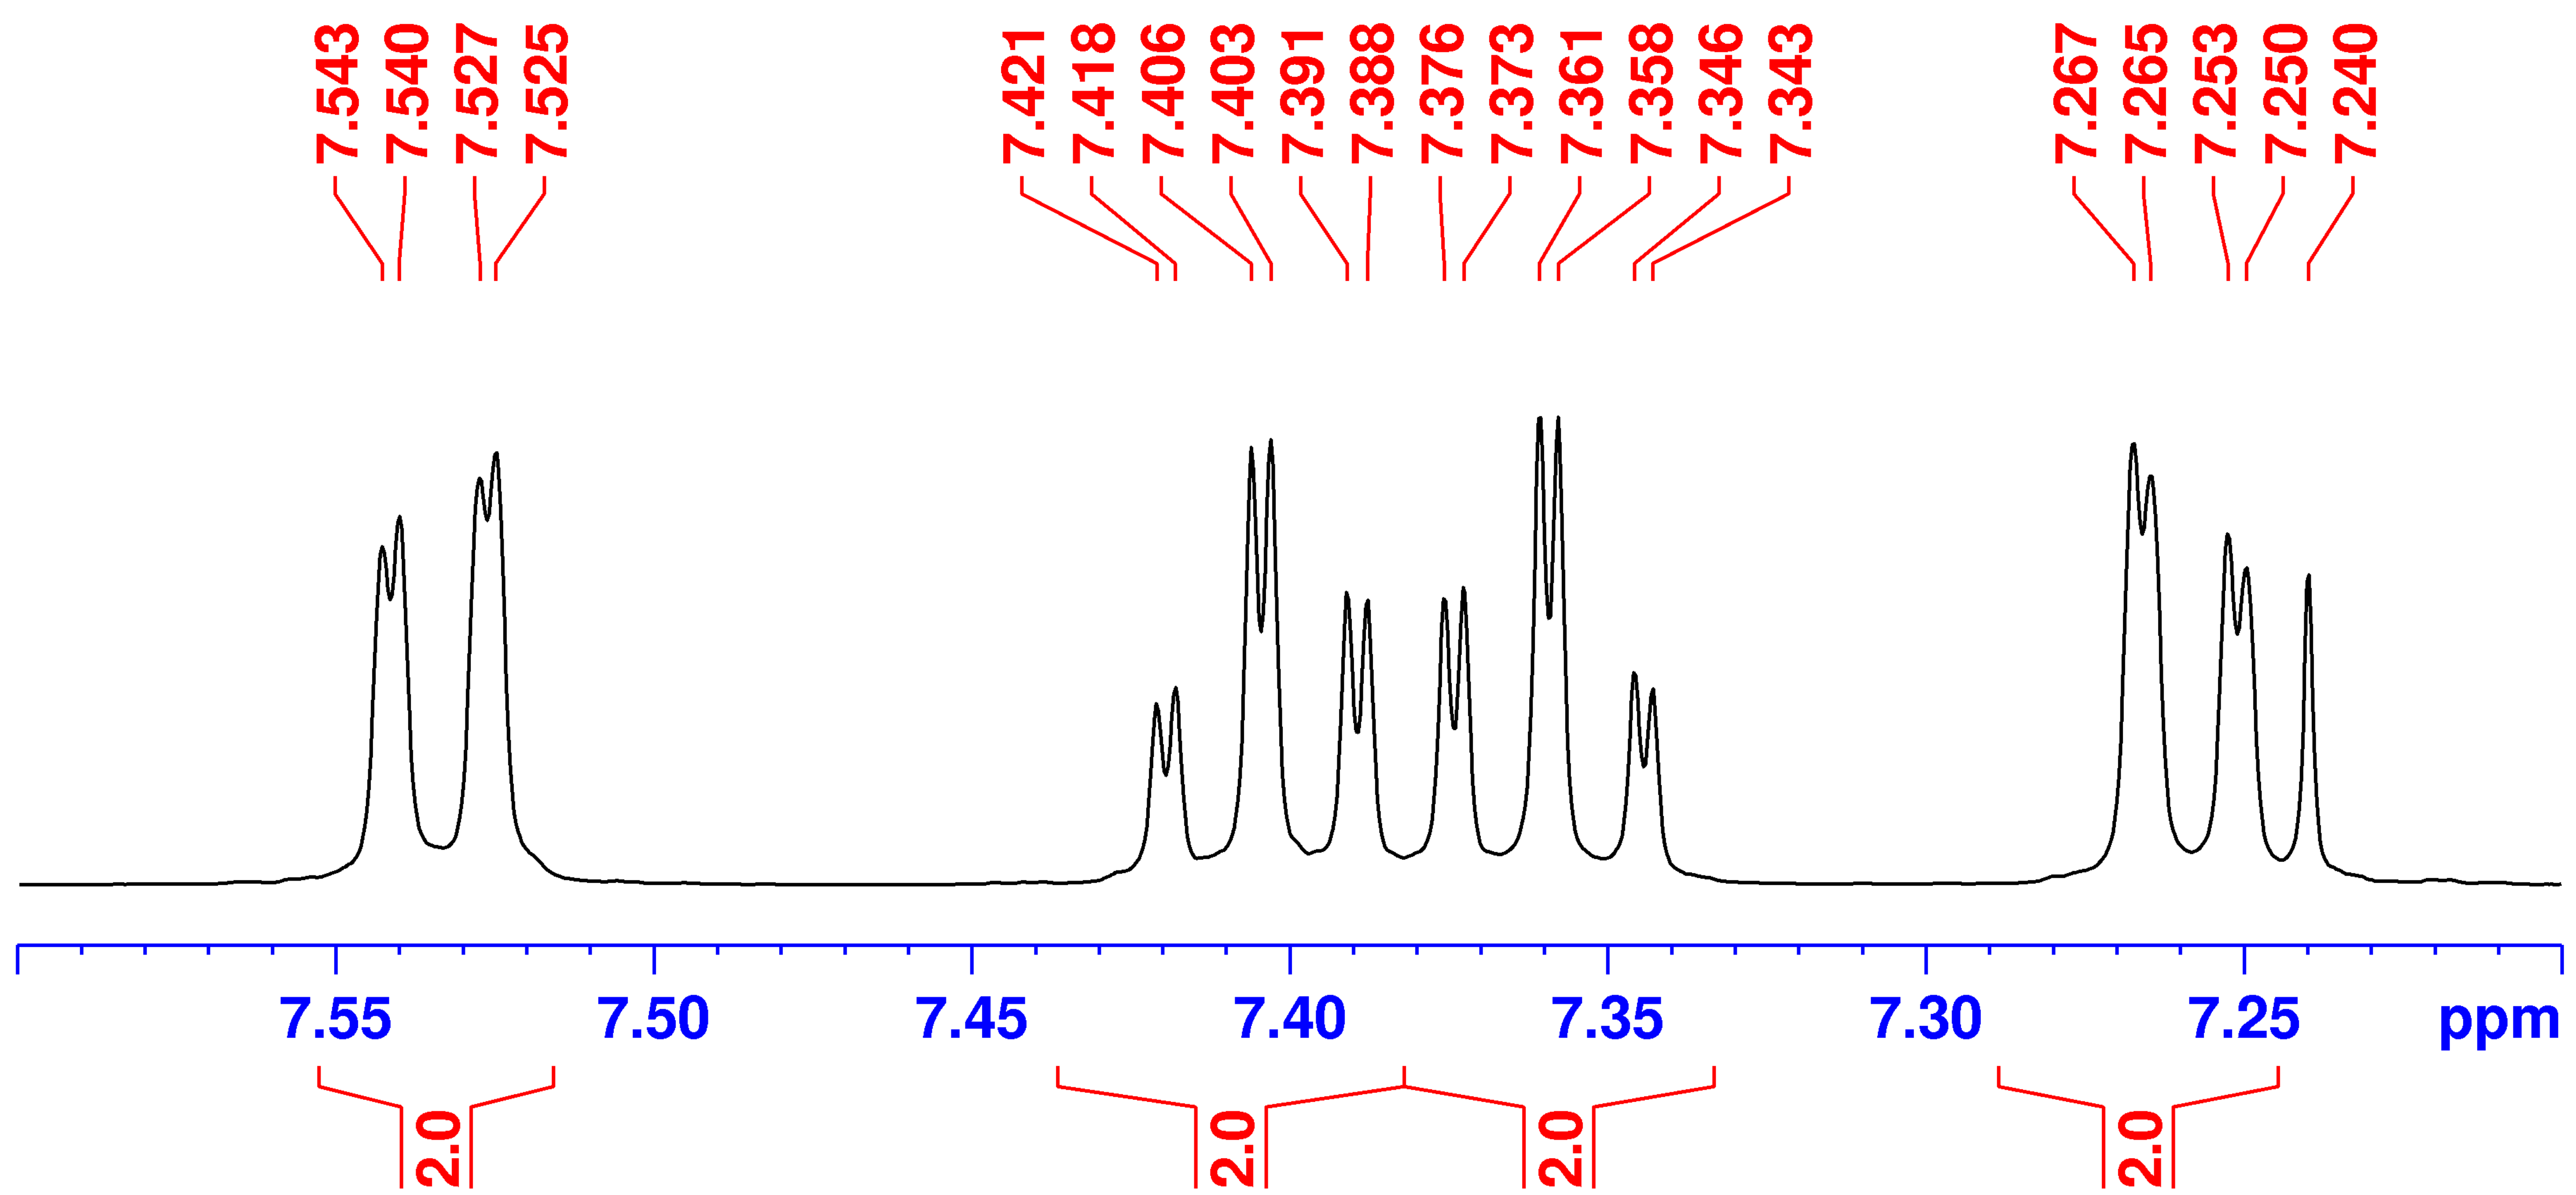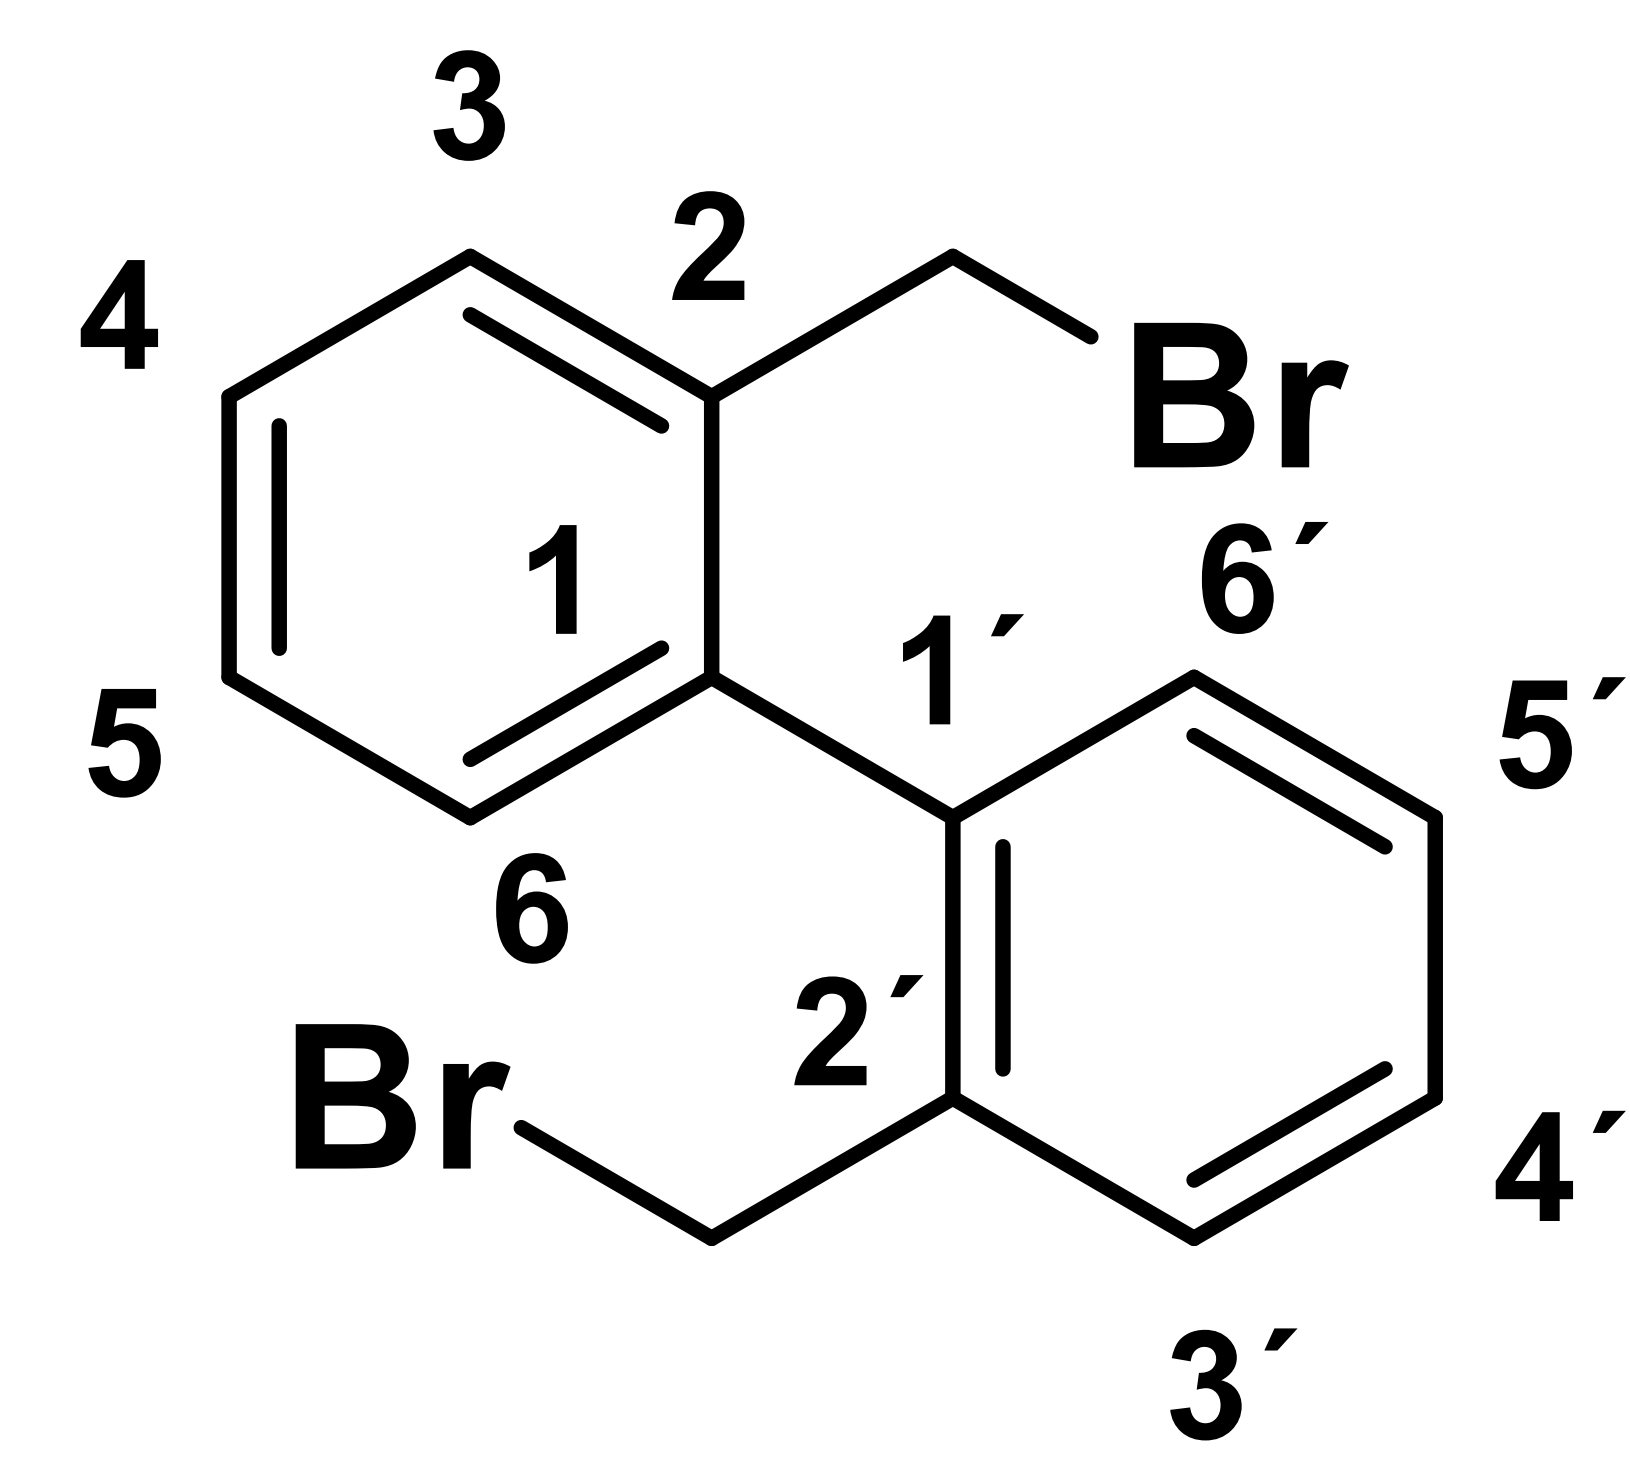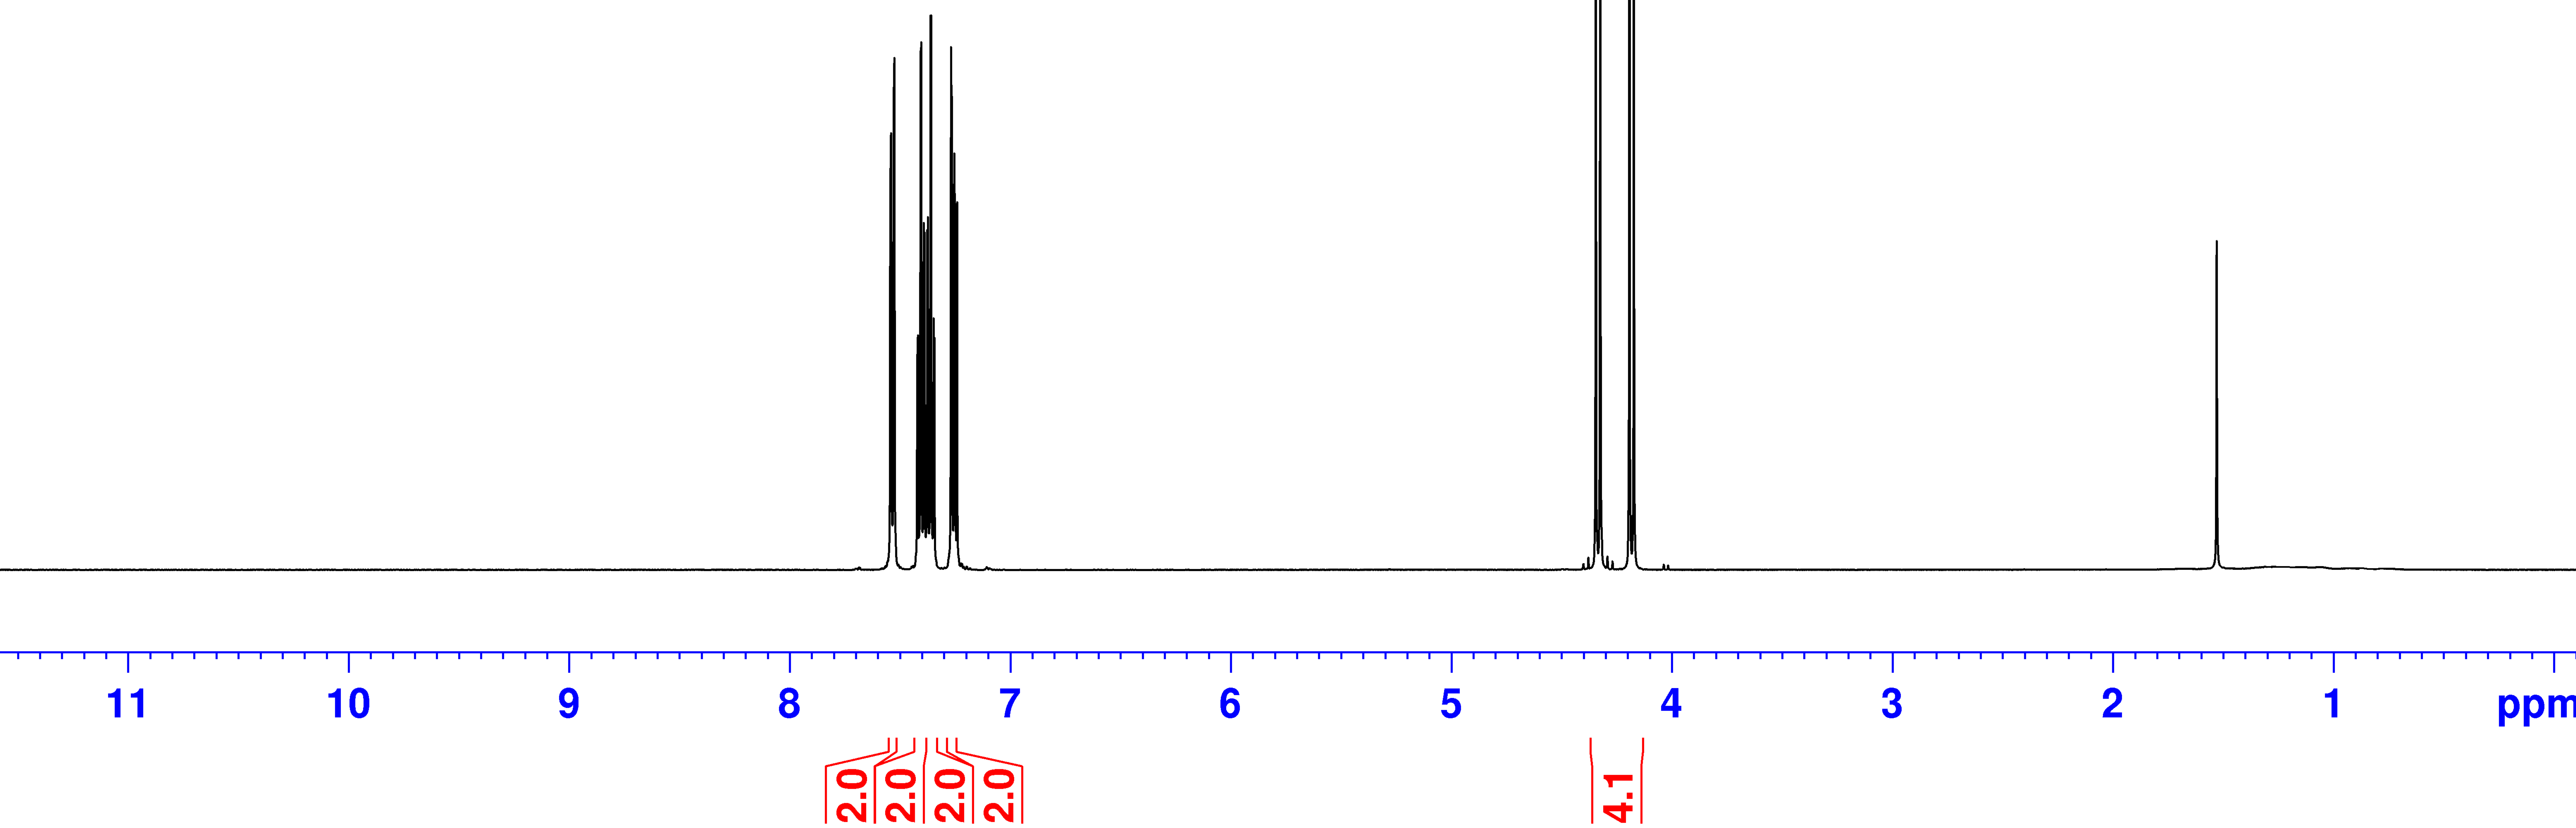

Supplement: Supplementary file 1 [file HNMR_III.pdf]
